# Supplementary material for: Learning an Unknown Network State in Routing Games
Source: arXiv:1905.04433 source file (2019-05-11)
Supplement: Supplementary file 1 [file appendix.tex]

%\begin{appendices}
%\renewcommand{\thesectiondis}[2]{\Alph{section}:}
%\section{Proof of Statements}\label{appendix}
%
%
%
%
%
%\vspace{0.2cm}
%
%\end{appendices}
